# Supplementary material for: Hybridization of lattice and charge order excitations in a superconducting cuprate
Source: arXiv:2503.20503 source file (2025-12-19)
Supplement: Supplementary file 1 [file SM.pdf]

# Supplemental Material for: Hybridization of lattice and charge order excitations in a superconducting cuprate

S. M. Souliou,[1,*] D. Ishikawa,[2,3] R. Heid,[1] D. Bessas,[4] H.H. Kim,[5] D. Betto,[5] S. Nakata,[5] M. Merz,[1,6] M. Minola,[5] B. Keimer,[5] A.Q.R. Baron,[2,3,†] and M. Le Tacon[1,‡]

[1]*Institute for Quantum Materials and Technologies, Karlsruhe Institute of Technology, Kaiserstr. 12, 76131 Karlsruhe, Germany*
[2]*Materials Dynamics Laboratory, RIKEN SPring-8 Center, Kouto 1-1-1, Sayo, Hyogo 679–5148, Japan*
[3]*Precision Spectroscopy Division, Japan Synchrotron Radiation Research Institute, Kouto 1-1-1, Sayo, Hyogo 679–5198, Japan*
[4]*ESRF, The European Synchrotron, 71, avenue des Martyrs, CS 40220 F-38043 Grenoble Cedex 9*
[5]*Max Planck Institute for Solid State Research, Heisenbergstraße 1, D-70569 Stuttgart, Germany*
[6]*Karlsruhe Nano Micro Facility (KNMFi), Karlsruhe Institute of Technology, 76344 Eggenstein-Leopoldshafen*
(Dated: March 26, 2025)

## S1. STRUCTURAL CHARACTERIZATION

X-ray diffraction (XRD) data on $YBa_2Cu_3O_{6.67}$ were collected at 295 K on a STOE imaging plate diffraction system (IPDS-2T) using Mo $K_\alpha$ radiation. All accessible symmetry-equivalent reflections were measured up to a maximum angle of $2\Theta = 65°$. The data were corrected for Lorentz, polarization, extinction, and absorption effects.

Using SHELXL [1] and JANA2006 [2], all accessed averaged symmetry-independent reflections ($I > 2\sigma$) have been included for the structure determination and for the corresponding refinement in the orthorhombic space group (SG) *Pmmm*. The oxygen content of $YBa_2Cu_3O_x$ was determined to $x = 6.66(3)$ and the twinning degree of the sample

| $YBa_2Cu_3O_{6.66(3)}$ | 295 K | | WP |
|---|---|---|---|
| | $a$ (Å) | 3.8220(4) | |
| | $b$ (Å) | 3.8795(3) | |
| | $c$ (Å) | 11.7109(8) | |
| | V (Å$^3$) | 173.643(2) | |
| Y | $U_{\mathrm{eqiv}}$ (Å$^2$) | 0.0039(2) | $1h$ |
| Ba | $z$ | 0.18735(3) | 2t |
| | $U_{\mathrm{eqiv}}$ (Å$^2$) | 0.0064(1) | |
| Cu(1) | $U_{\mathrm{eqiv}}$ (Å$^2$) | 0.0072(2) | $1a$ |
| Cu(2) | $z$ | 0.35653(6) | $2q$ |
| | $U_{\mathrm{eqiv}}$ (Å$^2$) | 0.0041(2) | |
| O(1) | $U_{\mathrm{eqiv}}$ (Å$^2$) | 0.0207(32) | $1e$ |
| O(2) | $z$ | 0.37915(36) | $2s$ |
| | $U_{\mathrm{eqiv}}$ (Å$^2$) | 0.0061(9) | |
| O(3) | $z$ | 0.37852(36) | $2r$ |
| | $U_{\mathrm{eqiv}}$ (Å$^2$) | 0.0054(9) | |
| O(4) | $z$ | 0.15645(37) | $2q$ |
| | $U_{\mathrm{eqiv}}$ (Å$^2$) | 0.0099(10) | |
| | GOF | 1.90 | |
| | $wR_2$ (%) | 4.57 | |
| | $R_1$ (%) | 1.94 | |
| | TW (%) | 97.5(8)/2.5(8) | |

Supplementary Table S-I. Crystallographic data for $YBa_2Cu_3O_{6.66(3)}$ at 295 K as determined from single-crystal XRD. The structure was refined in the orthorhombic space group *Pmmm*. Only the equivalent atomic displacement parameters $U_{\mathrm{eqiv}}$ are listed, while the anisotropic atomic displacement parameters were used for the refinement. The corresponding Wyckoff positions (WP) are given as well. TW represents the degree of twinning determined from the refinement. Errors shown are statistical errors from the refinement.

* michaela.souliou@kit.edu
† baron@spring8.or.jp
‡ matthieu.letacon@kit.edu

to 97.5/2.5 %. The refinement converged quite well and shows excellent reliability factors (see GOF, R1, and wR2 in Table S1).

## S2. DENSITY FUNCTIONAL THEORY CALCULATIONS

Phonon properties, i. e. frequencies and eigenvectors, which are required for the calculation of the IXS structure factor, were obtained using linear response or density functional perturbation theory. Here we briefly outline the main aspects, while more technical details have been already described in previous publications [3, 4]. We employed an implementation of the density-functional perturbation theory in the so-called mixed-basis method [5, 6]. In this approach valence states are expanded in a basis set consisting of a combination of plane waves and local functions. The latter allow an efficient description of more localized components of the valence states. Here, plane waves up to a kinetic energy of 20 Ry, augmented by local functions of $s$,$p$,$d$ type at the Y and Ba sites, of $s$ and $p$ type at the O sites and of $d$ type at the Cu sites were used. The electron-ion interaction was represented by norm-conserving pseudopotentials, which included the semi-core states Y-4$s$, Y-4$p$, Ba-5$s$, Ba-5$p$, and O-2$s$ in the valence space. Calculations were carried out for the fully oxygenated $YBa_2Cu_3O_7$ employing the local-density approximation [7]. For Brillouin zone integrations a 12x12x4 k-point grid in conjunction with a Gaussian smearing of 0.2 eV was used. Dynamical matrices were calculated on a 4x4x2 momentum grid, and then determined for arbitrary points in the Brillouin zone by standard Fourier-interpolation techniques.

Calculated dispersions and structure factors along the $L$ direction and across the reciprocal space positions corresponding to the spectra plotted in Fig.3 of the main text are shown in Fig.S1. $L$=7 and $L$=1 in panels Fig.S1-(c) and (d) correspond to $\mathbf{Q}_{\mathbf{3D}}^{\mathbf{trans}}$ and $\mathbf{Q}_{\mathbf{3D}}^{\mathbf{long}}$ respectively. The results remain qualitatively very similar when moving a bit

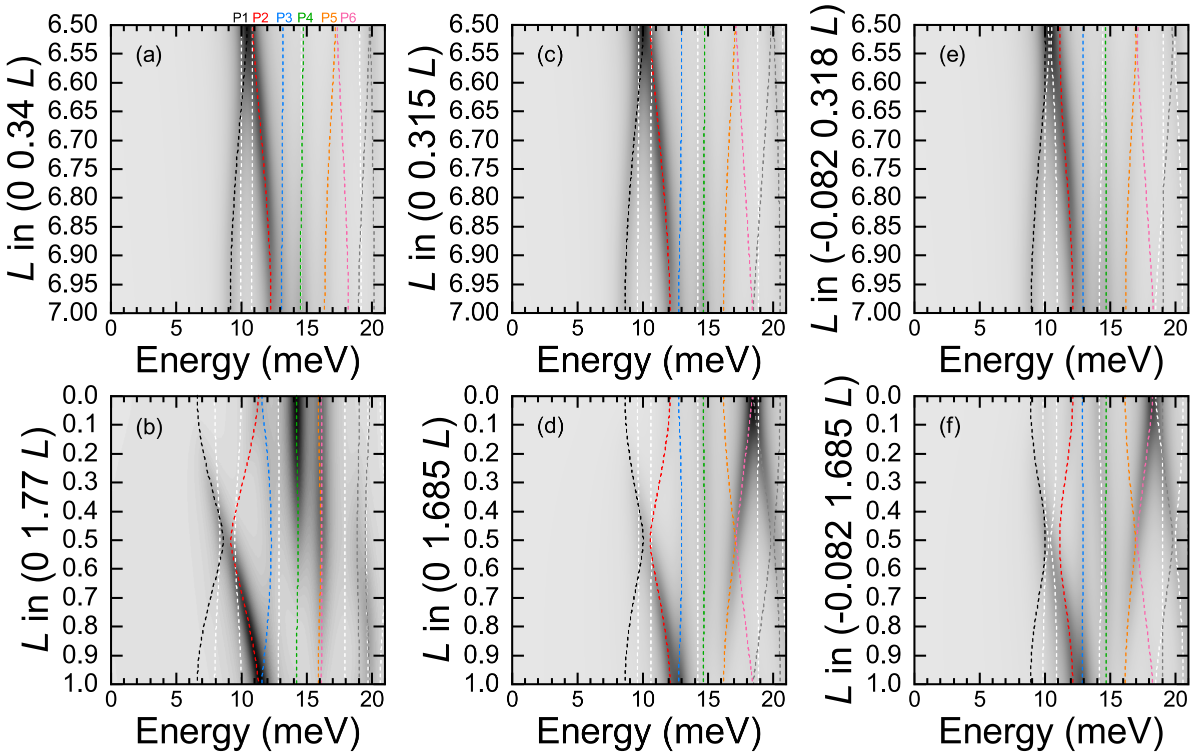


Supplementary Figure S1. Phonon dispersion curves of $YBa_2Cu_3O_7$ along (a) (0 0.34 $L$), (b) (0 1.77 $L$), (c) (0 0.315 $L$), (d) (0 1.685 $L$), (e) (-0.082 0.318 $L$) and (f) (-0.082 1.685 $L$) calculated by density-functional perturbation theory. The phonon branches are grouped in two categories based on the symmetry operations for their displacement patterns: the first category (colored/grey lines) includes a mirror symmetry operation ($\sigma(x)$, $x \to -x$), whereas the second category (white lines) does not. Further symmetry operations are restored for the displacement patterns of some of the modes at integer and half-integer $L$. The calculations of panel (d) are the same as those shown in Fig.2 of the main text. A colormap representation of the calculated structure factors is shown in the background of all panels using a common scale.

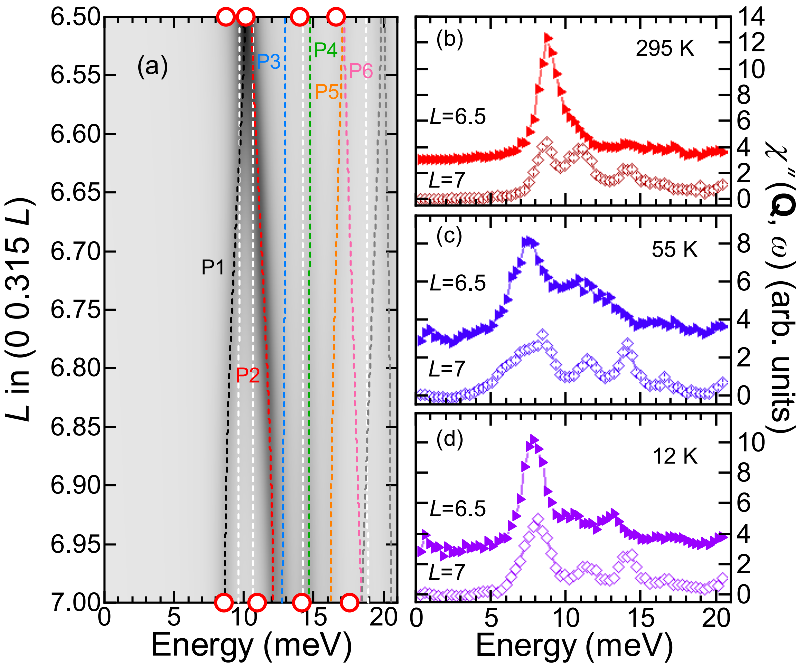


Supplementary Figure S2. (a) Phonon dispersion curves of $YBa_2Cu_3O_7$ along (0 0.315 $L$) calculated by density-functional perturbation theory. A colormap representation of the calculated structure factors is shown in the background. The coloring of the dispersion curves and the colormap scaling is the same as in Fig.S1. (b-d) $L$ dependence of $\chi''(\boldsymbol{Q},\omega)$ at (b) 295 K, (c) 55 K and (d) 12 K. The spectra have been shifted vertically for clarity.

away from $\mathbf{Q}_{\mathbf{3D}}^{\mathbf{trans}}$ and $\mathbf{Q}_{\mathbf{3D}}^{\mathbf{long}}$ along the $K$ (Fig.S1-(a) and (b)) and $H$ directions (Fig.S1-(e) and (f)), both in terms of the expected scattering intensity and of the phonon dispersions and intersection effects. These results speak against phonon-phonon anti-crossings being the origin of the phonon anomalies observed experimentally at $\mathbf{Q}_{\mathbf{3D}}^{\mathbf{trans}}$ and $\mathbf{Q}_{\mathbf{3D}}^{\mathbf{long}}$ and presented in the main text.

## S3. $L$ DEPENDENCE OF THE IXS SPECTRA IN THE TRANSVERSE GEOMETRY

The $L$ and temperature dependence of the IXS spectra in the transverse geometry is presented in Fig.S2, together with the calculated phonon dispersions and structure factors in the used Brillouin zone. Similar to the observations in the longitudinal geometry presented in Fig.2 of the main text, additional spectral weight appears at low temperatures both at $\mathbf{Q}_{\mathbf{3D}}^{\mathbf{trans}}$ and at $\mathbf{Q}_{\mathbf{2D}}^{\mathbf{trans}}$. The observed phonon anomalies at $\mathbf{Q}_{\mathbf{3D}}^{\mathbf{trans}}$, but also at $\mathbf{Q}_{\mathbf{2D}}^{\mathbf{trans}}$, cannot be explained solely by a phonon softening of the acoustic phonon P1, as postulated in earlier studies with lower energy resolution [4, 8].

## S4. IXS SPECTRA AT $\boldsymbol{Q}$ = (0 1.685 0) AND $\boldsymbol{Q}$ = (0 3.685 1)

The IXS spectra recorded at $\boldsymbol{Q}$ = (0 1.685 0) are presented in Fig.S3. Three peaks are clearly visible, in good agreement with the calculations (see Fig.S1-(d)) which predict contributions from the P2, P4 and P6 modes. The spectra remain almost unchanged from 295 to 12 K. This is unlike the IXS spectra at $L$=1, i.e. at $\mathbf{Q}_{\mathbf{3D}}^{\mathbf{long}}$, presented in the main text, where the calculations predict contributions mostly from the P2 and P3 modes.

According to our structure factor calculations, the P2 and P3 modes also contribute to the scattered intensity at $\boldsymbol{Q}$ = (0 3.685 1). The recorded spectra are presented in Fig.S4. While one peak at ∼11 meV is observed at room temperature, (at least) three distinct features at ∼7.5, 11, and 14 meV are present in the 12 K spectrum. Overall, the experimental observations are very similar to the ones at $\mathbf{Q}_{\mathbf{3D}}^{\mathbf{long}}$ (also shown in Fig.S4 for direct comparison).

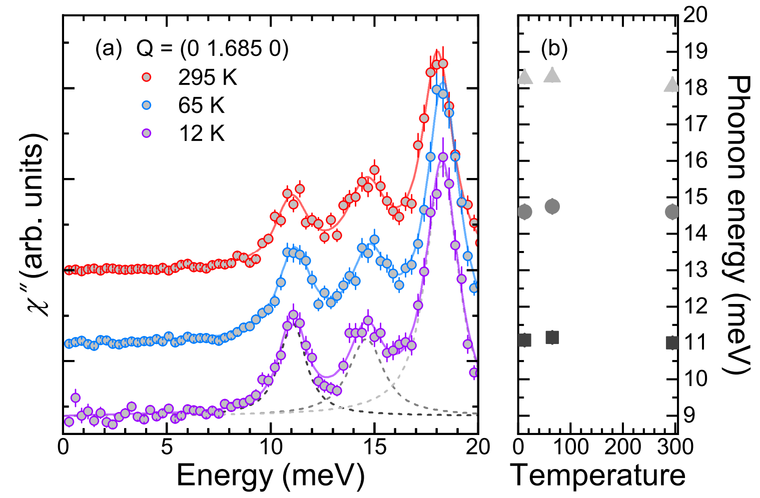


Supplementary Figure S3. (a) Temperature dependence of $\chi''(\boldsymbol{Q},\omega)$ at $\boldsymbol{Q} = (0\ 1.685\ 0)$. The spectra have been shifted vertically for clarity. (b) Temperature dependence of the P2, P4 and P6 phonon energies extracted from the fits.

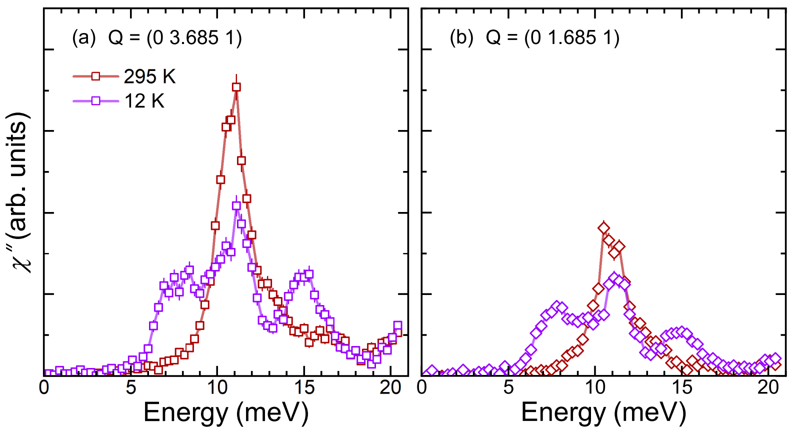


Supplementary Figure S4. $\chi''(\boldsymbol{Q},\omega)$ at (a) $\boldsymbol{Q}$= (0 3.685 1) and (b) $\boldsymbol{Q}$= (0 1.685 1) at room and base temperature. The vertical axis scale is common in the two panels.

## S5. PHONON ANALYSIS

Fig.S5 displays details of fits of the IXS spectra at $\mathbf{Q}_{\mathbf{3D}}^{\mathbf{long}}$ at 295, 55 K and at 12 K. The fits were performed using a resolution limited elastic line and damped harmonic oscillator (DHO) lineshapes (convoluted with the experimental resolution function) for the phonons. The resolution was determined using Plexiglas measurements. As discussed in the main text, the room temperature spectrum is dominated by a single peak at ∼11 meV. The peak appears asymmetric and a better fit of the data is achieved when including two DHO lineshapes, one main peak centered at ∼10.8 meV and a second side-peak at ∼12.7 meV (Fig.S5-(a,b)). At low temperatures, (at least) three distinct features are observed. Including one additional DHO (at ∼7.9 meV) appears insufficient to account for the additional features appearing at low temperatures (Fig.S5-(c,e)) and a better fit is achieved when including two additional DHOs (∼7.6 meV and ∼9.3 meV, see Fig.S5-(d,f)), highlighting the unusual lineshape of the low temperature spectral weight.

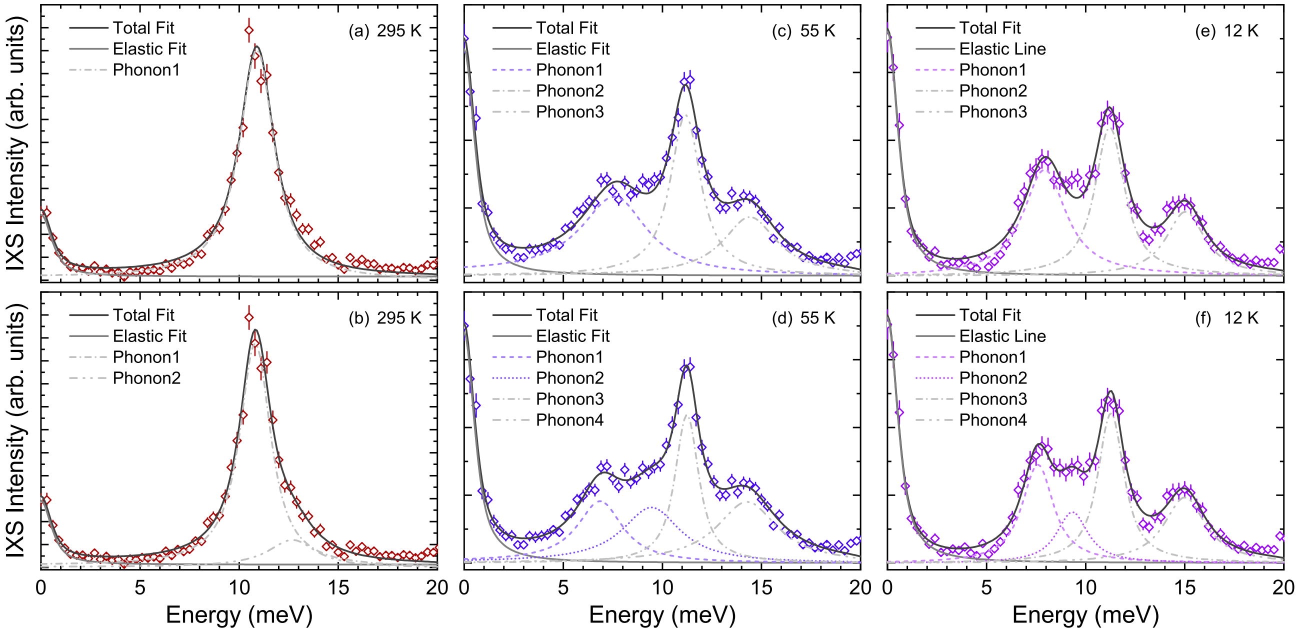


Supplementary Figure S5. Details of the fit of the IXS spectra at $\mathbf{Q}_{\mathbf{3D}}^{\mathbf{long}}$ at 295, 55 and 12 K following the procedure described in the text. The y-axis scale is not common to all panels.

## S6. IXS SPECTRA FROM THE FULL ANALYSERS' ARRAY

Fig.S6 and Fig.S7 display the temperature dependence of the IXS spectra recorded simultaneously in the 2-dimensional array of $7 \times 4 = 28$ analyzers. The large array helped to make the specific q-dependence of the observed low temperature effects very clear as only the central analyser positioned at $\mathbf{Q}_{\mathbf{3D}}^{\mathbf{long}}$ (Fig.S6) and at $\mathbf{Q}_{\mathbf{3D}}^{\mathbf{trans}}$ (Fig.S7) respectively shows strong temperature dependence (after scaling by the Bose factor), and the rest of the 2D array showed no significant changes.


[1] G. M. Sheldrick, Acta Crystallogr. Sect. A **64**, 112 (2008).
[2] V. Petříček, M. Dušek, and L. Palatinus, Z. Kristallogr. Cryst. Mater. **229**, 345 (2014).
[3] S.-M. Souliou, K. Sen, R. Heid, S. Nakata, L. Wang, H.-h. Kim, H. Uchiyama, M. Merz, M. Minola, B. Keimer, and M. Le Tacon, J. Phys. Soc. Jpn. **90**, 111006 (2021).
[4] H.-H. Kim, S. M. Souliou, M. E. Barber, E. Lefrançois, M. Minola, M. Tortora, R. Heid, N. Nandi, R. A. Borzi, G. Garbarino, A. Bosak, J. Porras, T. Loew, M. König, P. J. W. Moll, A. P. Mackenzie, B. Keimer, C. W. Hicks, and M. Le Tacon, Science **362**, 1040 (2018).
[5] B. Meyer, C. Elsässer, F. Lechermann, and M. Fähnle, Max-Planck-Institut für Metallforschung, Stuttgart (unpublished).
[6] R. Heid and K. P. Bohnen, Phys. Rev. B **60**, R3709 (1999).
[7] L. Hedin and B. I. Lundqvist, Journal of Physics C: Solid State Physics **4**, 2064 (1971).
[8] M. Le Tacon, A. Bosak, S. M. Souliou, G. Dellea, T. Loew, R. Heid, K.-P. Bohnen, G. Ghiringhelli, M. Krisch, and B. Keimer, Nat. Phys. **10**, 52 (2014).

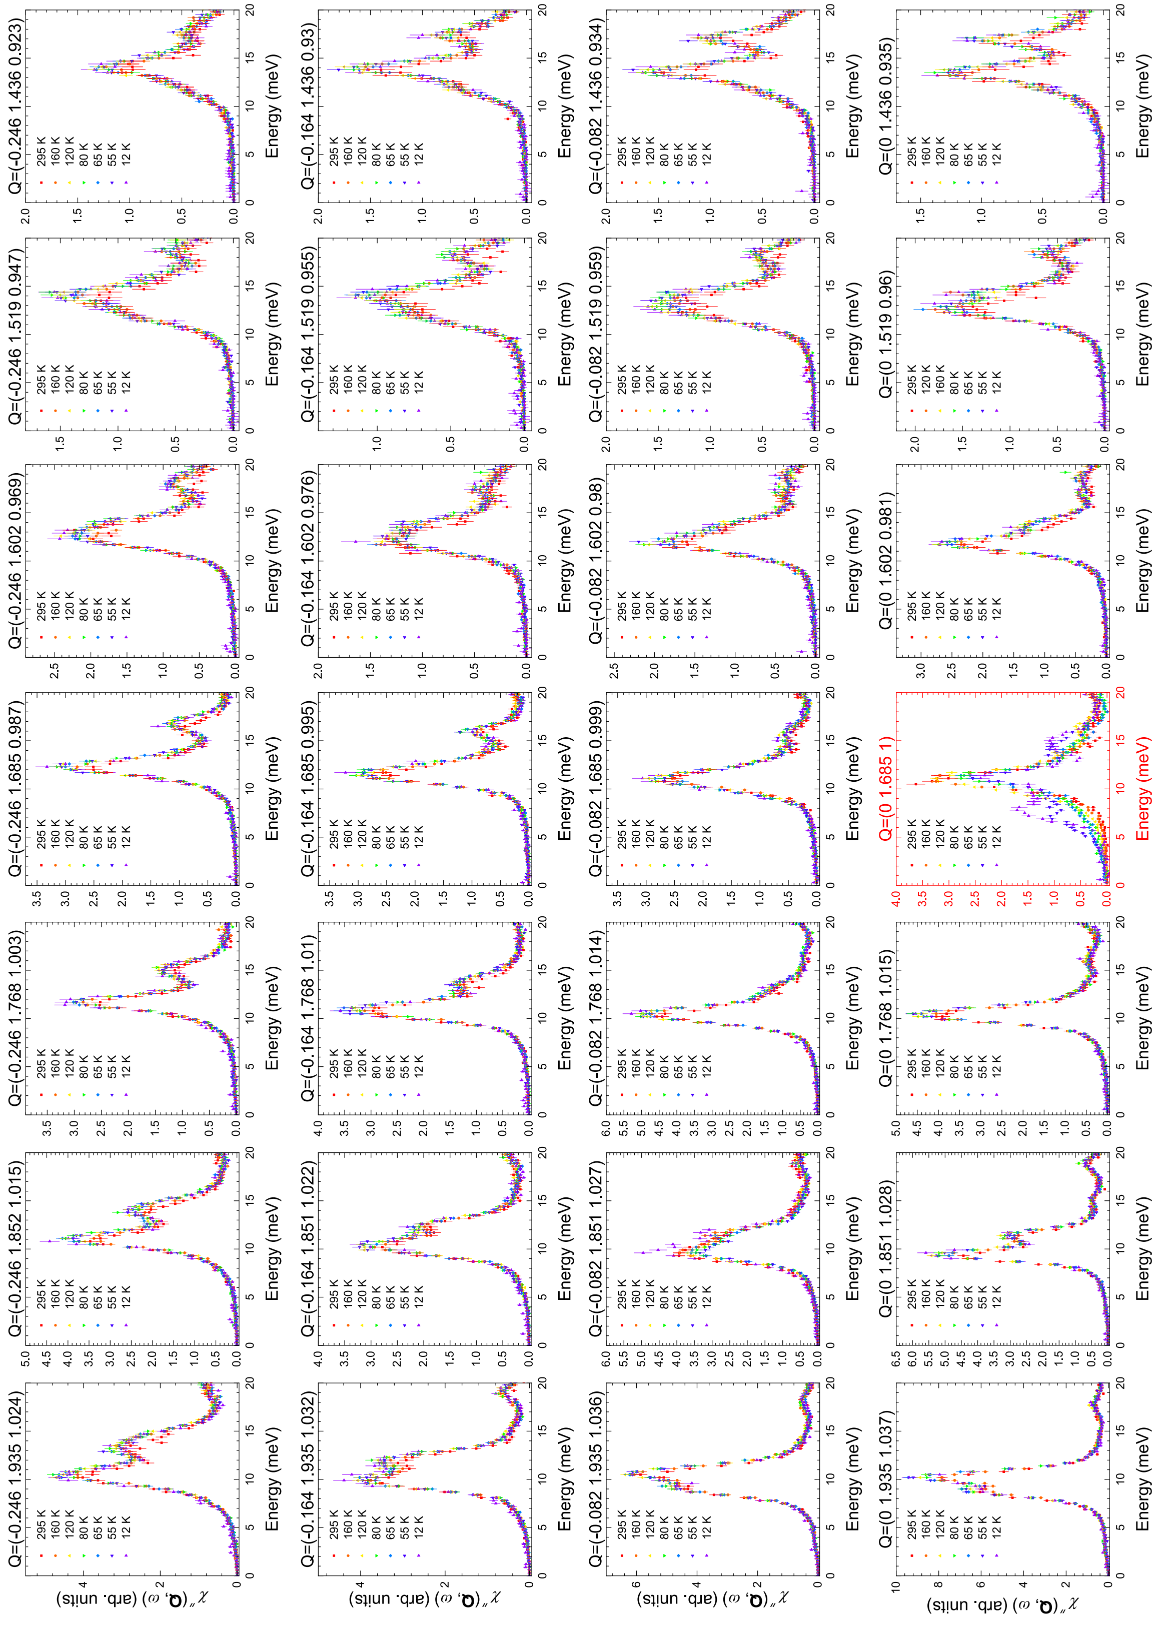


Supplementary Figure S6. Temperature dependence of the IXS spectra recorded simultaneously in the full array of analysers. The central analyser is positioned at $\mathbf{Q}_{\mathbf{3D}}^{\mathbf{long}}$ and is highlighted in red.

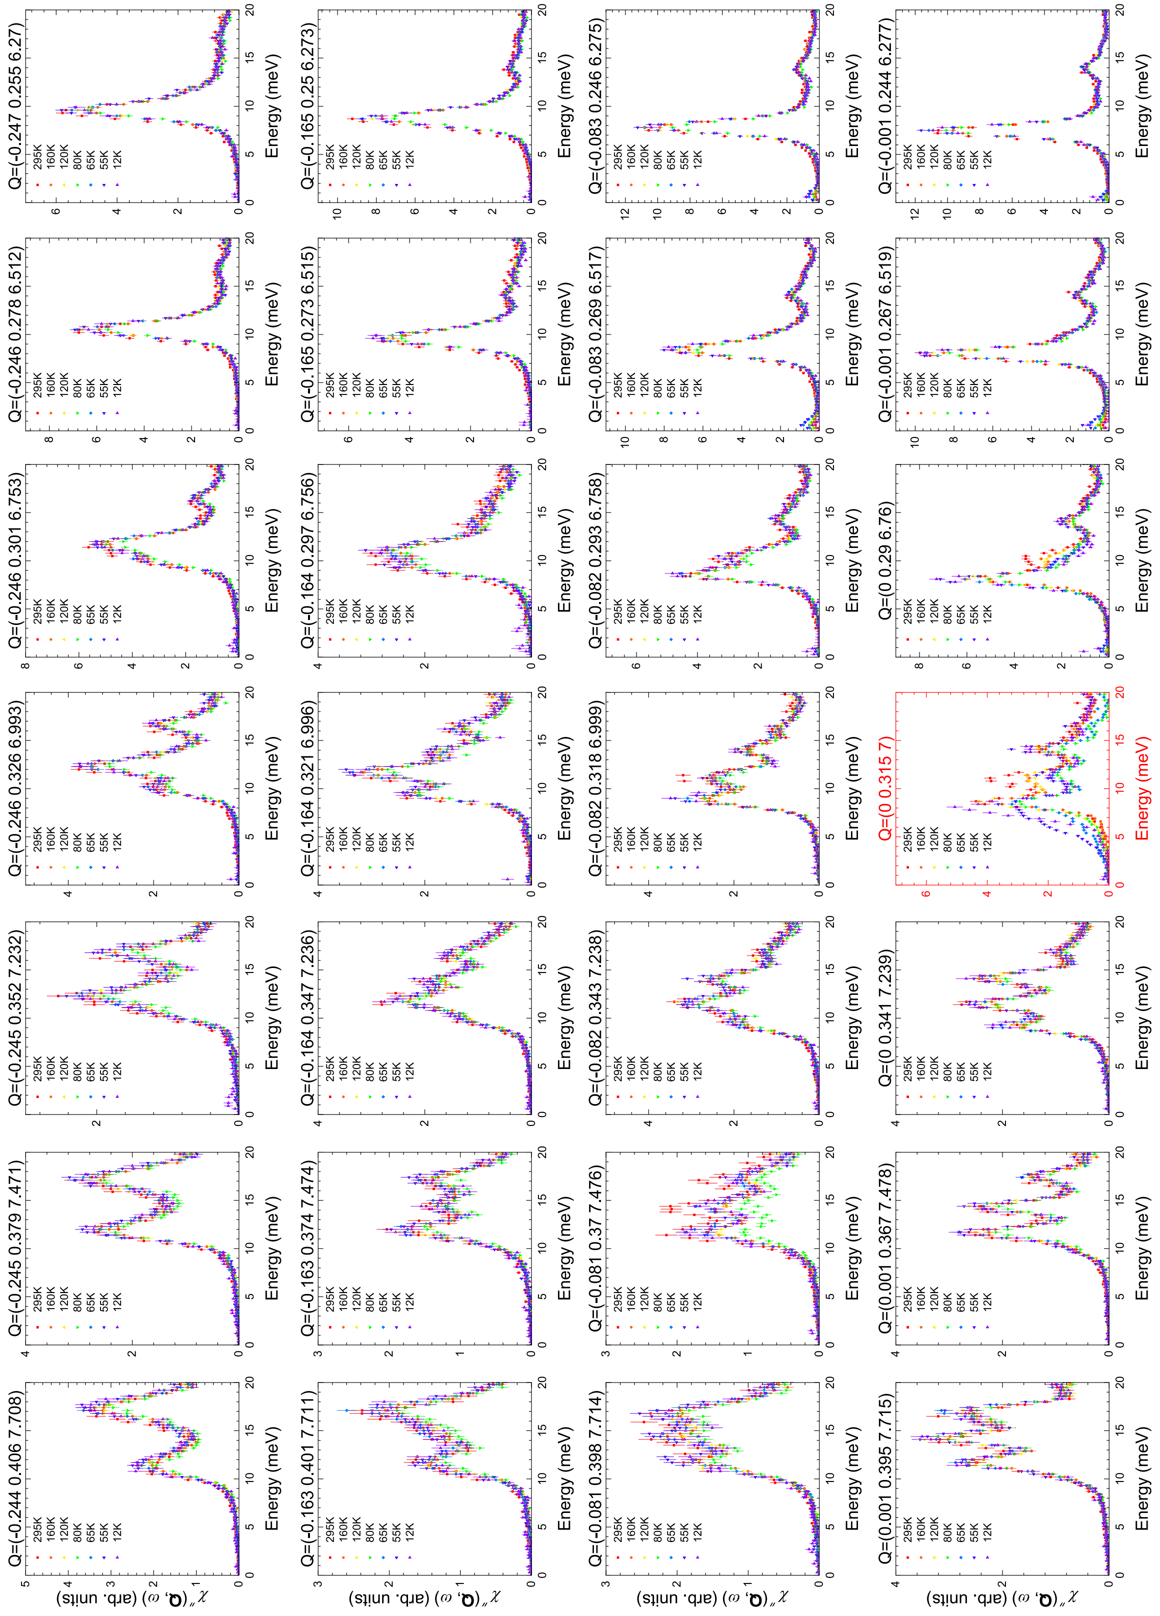


Supplementary Figure S7. Temperature dependence of the IXS spectra recorded simultaneously in the full array of analysers. The central analyser is positioned at $\mathbf{Q}_{\mathbf{3D}}^{\mathbf{trans}}$ and is highlighted in red.
